# Supplementary material for: Stabilizing Linear Systems under Partial Observability: Sample Complexity and Fundamental Limits
Source: arXiv:2503.16756 source file (2025-03-21)
Supplement: Supplementary file 1 [file appendix_index.tex]

For the convenience of readers, we provide a table summarizing all constants appearing in the bounds. 
\begin{table}[!htbp]
\caption{Lists of parameters and constants appearing in the bound.}
\label{table:algorithm}
\vskip 0.15in
\begin{center}
\begin{small}
\begin{tabular}{lcccr}
\toprule
\textbf{Constant} & \textbf{Appearance} & \textbf{Explanation} \\
\midrule
$T$    & \Cref{sec:intro} & Length of each roll out. \\
$M$ & \Cref{sec:alg_dev} & Number of roll outs.\\
$m$ & \Cref{sec:alg_dev} & number of open-loop steps for converging to unstable state space. 
\\
$p,q$ & \Cref{sec:alg_dev} & dimension of Hankel matrix to be estimated. 
         \\
\bottomrule
\end{tabular}
\end{small}
\end{center}
\vskip -0.1 in
\caption{System theoretic parameters.}
\label{table:parameters}
\vskip 0.15in
\begin{center}
\begin{small}
\begin{tabular}{lcccr}
\toprule
\textbf{Constant} & \textbf{Appearance} & \textbf{Explanation} \\
\midrule
$\Tilde{o}_{\min}(m)$    & \Cref{lemm:OC_bnd} & a positive real number such that $\sigma_{\min}(\tilde{\cO}) \geq \Tilde{o}_{\min}(m)$.\\
$\tilde{c}_{\min}(m)$ & \Cref{lemm:OC_bnd} & a positive real number such that $\sigma_{\min}(\tilde{C}) \geq \tilde{c}_{\min}(m)$.
\\
$\alpha$    & \Cref{appendix:Hankel} & Controllability index.\\
$C_C,C_B$    & \eqref{eqn:CcCb} & modified controllability and observability matrices.
\\
$\zeta_{\epsilon}(\cdot)$ & \Cref{lemma:Gelfand} & Gelfand constant for the norm of matrix exponents \\
\bottomrule
\end{tabular}
\end{small}
\end{center}

\vskip -0.1 in
\caption{Shorthand notations (introduced in proofs).}
\label{table:shorthand}
\vskip 0.15in
\begin{center}
\begin{small}
\begin{tabular}{lcccr}
\toprule
\textbf{Constant} & \textbf{Appearance} & \textbf{Explanation} \\
\midrule
$\underline{\sigma}_s$ & \Cref{lemm:OC_bnd} & $\underline{\sigma}_s := \frac{\sigma_{\min}(C_c)}{\sigma_{\max}(C_B)}$
\\
$\overline{\sigma}_s$ & \Cref{lemm:OC_bnd} & $\overline{\sigma}_s := \frac{\sigma_{\max}(C_c)}{\sigma_{\min}(C_B)}$
\\
$\epsilon_N$ & \Cref{lemm:bnd_N1} & $\epsilon_N := \frac{2\left(1+\zeta_{\epsilon_1}(N_1)(\lambda_1+\epsilon_1)\right)c_2\epsilon}{c_1 \sigma_{\min}(\tilde{\cO})}$
\\
$\epsilon_C$ & \Cref{lemm:C_hat_bnd} & $\epsilon_C := 2\Big(\frac{4c_2\norm{CQ_1}}{c_1\sigma_{\min}(\tilde{\cO})}+\frac{1}{\sigma_{\min}(\tilde{\cC})}\Big)\epsilon$
\\
$\epsilon_B$ & \Cref{lemm:B_hat_bnd} & $\epsilon_B := 8\left(\frac{c_2\norm{R_1B}}{c_1\sigma_{\min}(\tilde{\cC})} + \frac{1}{\sigma_{\min}(\tilde{O})}\right)\epsilon$
\\
$\epsilon_*$ & \Cref{assumption:F_bnd} & 
\\
$\epsilon$ & \Cref{lemm:hankel_bnd} & $\epsilon := \hat{\epsilon} + \bar{\epsilon} +\tilde{\epsilon}$
\\
$\tilde{\epsilon}$ & \Cref{lemm:bdd_H_tildeH} & $\tilde{\epsilon}:= \sqrt{q}p\norm{B}\norm{C}\zeta_{\epsilon_2}(N_2)(\lambda_{k+1}+\epsilon_2)^{m}$
\\
$\hat{\epsilon}$ & \Cref{lemm:hankel_bnd} & $\hat{\epsilon}:= \frac{8\sigma_{v} \sqrt{T(T+1)(d_u+d_y)\max\{p,q\}\log(27T/\delta)}}{\sigma_u \sqrt{M}}$
\\
\bottomrule
\end{tabular}
\end{small}
\end{center}
\end{table}
